# Supplementary material for: Stubborn: A Strong Baseline for Indoor Object Navigation
Source: arXiv:2203.07359 source file (2022-03-14)
Supplement: Supplementary file 1 [file appendix.tex]

\appendix

We present implementation details related to the Object Detection Module (Section \ref{ODM}) below.

\noindent
\textbf{Definition of Object} An object in a human's concept, such as a bed or a table, usually corresponds to multiple grid points that are next to each other on the 2D grid map. Therefore, we treat each connected component of the non-zero entries of Channel 6 (maximum confidence channel) as an object.

\noindent
\textbf{Object Feature Vector}

The Point Set, $P_O$, is the collection of coordinates belonging to the object $O$ in the global map $\mathcal{M}$:

P_O&\coloneqq \SET{(i,j)}{$(i,j)$ belongs to the Object $O$}

The Map, $M$, is the global map defined in Sec. \ref{mapping}. The first two dimensions of $M$ are the coordinates of the grid, and the third dimension of $M$ is the channel presented in Table \ref{tab:map}. 

Details on the $5$ dimensions of the feature vector is described below.

\begin{itemize}
\item \textbf{Maximum Confidence Score} This is the maximum confidence score reported by the segmentation model for the candidate object:
$$
\max_{(i,j)\in P_O} M_{(i,j,6)}
$$
    \item \textbf{Cumulative Confidence Score} This is the sum of confidence scores of the candidate object across all the frames:
$$
\max_{(i,j)\in P_O} M_{(i,j,5)}
$$
    \item \textbf{Total Number of Frames} This is the total number of frames the candidate object appeared in the view of the agent, regardless of whether the candidate object is identified as a goal or not by the semantic segmentation model:
$$
\max_{(i,j)\in P_O} M_{(i,j,4)}
$$
    \item \textbf{Average Confidence Score} This is the average confidence score of the candidate among all the frames it appeared in the view of the agent:
$$
\max_{(i,j)\in P_O} \frac{M_{(i,j,5)}}{M_{(i,j,4)}}
$$
    \item \textbf{Conflict Object Score} It is the highest confidence score of non-goal categories reported by the semantic segmentation model in the same location of the goal candidate object:
$$
\max_{(i,j)\in P_O} M_{(i,j,7)}
$$
\end{itemize}
